# Supplementary material for: Query Rewriting with Disjunctive Existential Rules and Mappings
Source: arXiv:2306.05973 source file (2023-06-09)
Supplement: Supplementary file 1 [file appendix.tex]

\appendix
